# Supplementary material for: Computing Electronic Correlation Energies using Linear Depth Quantum Circuits
Source: arXiv:2207.03949 source file (2022-08-09)
Supplement: Supplementary file 1 [file appendix_cropped.pdf]

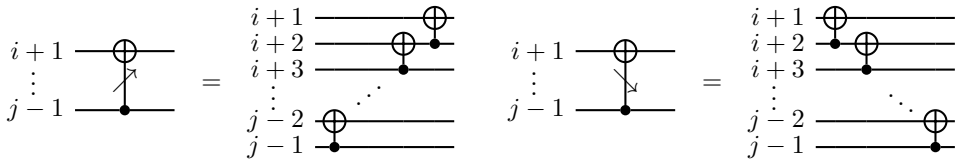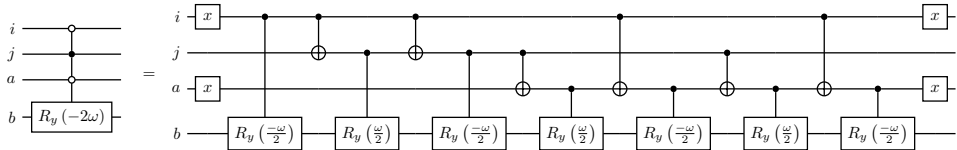

Orbital energy  
levels not to scale.

Grey: Inactive

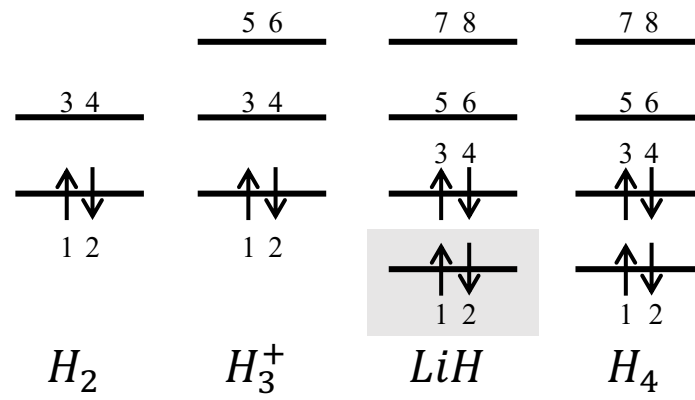

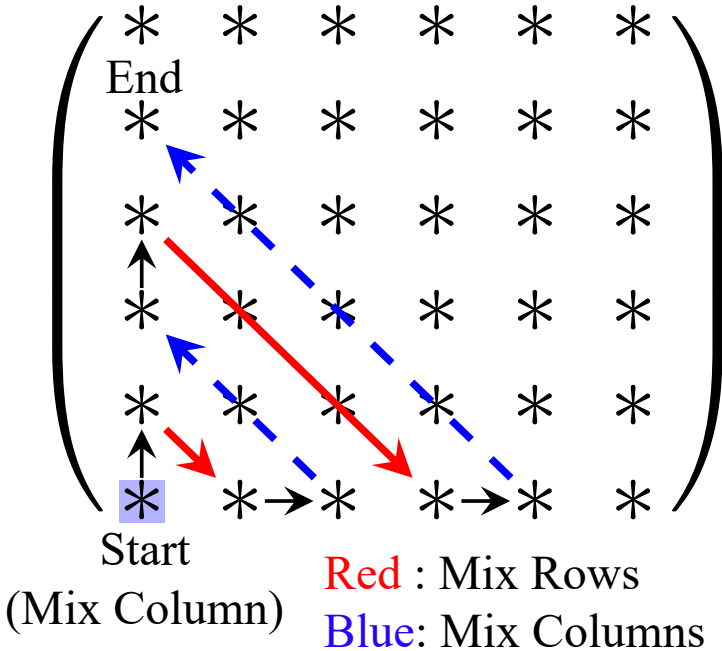

# Simulated IBM Auckland

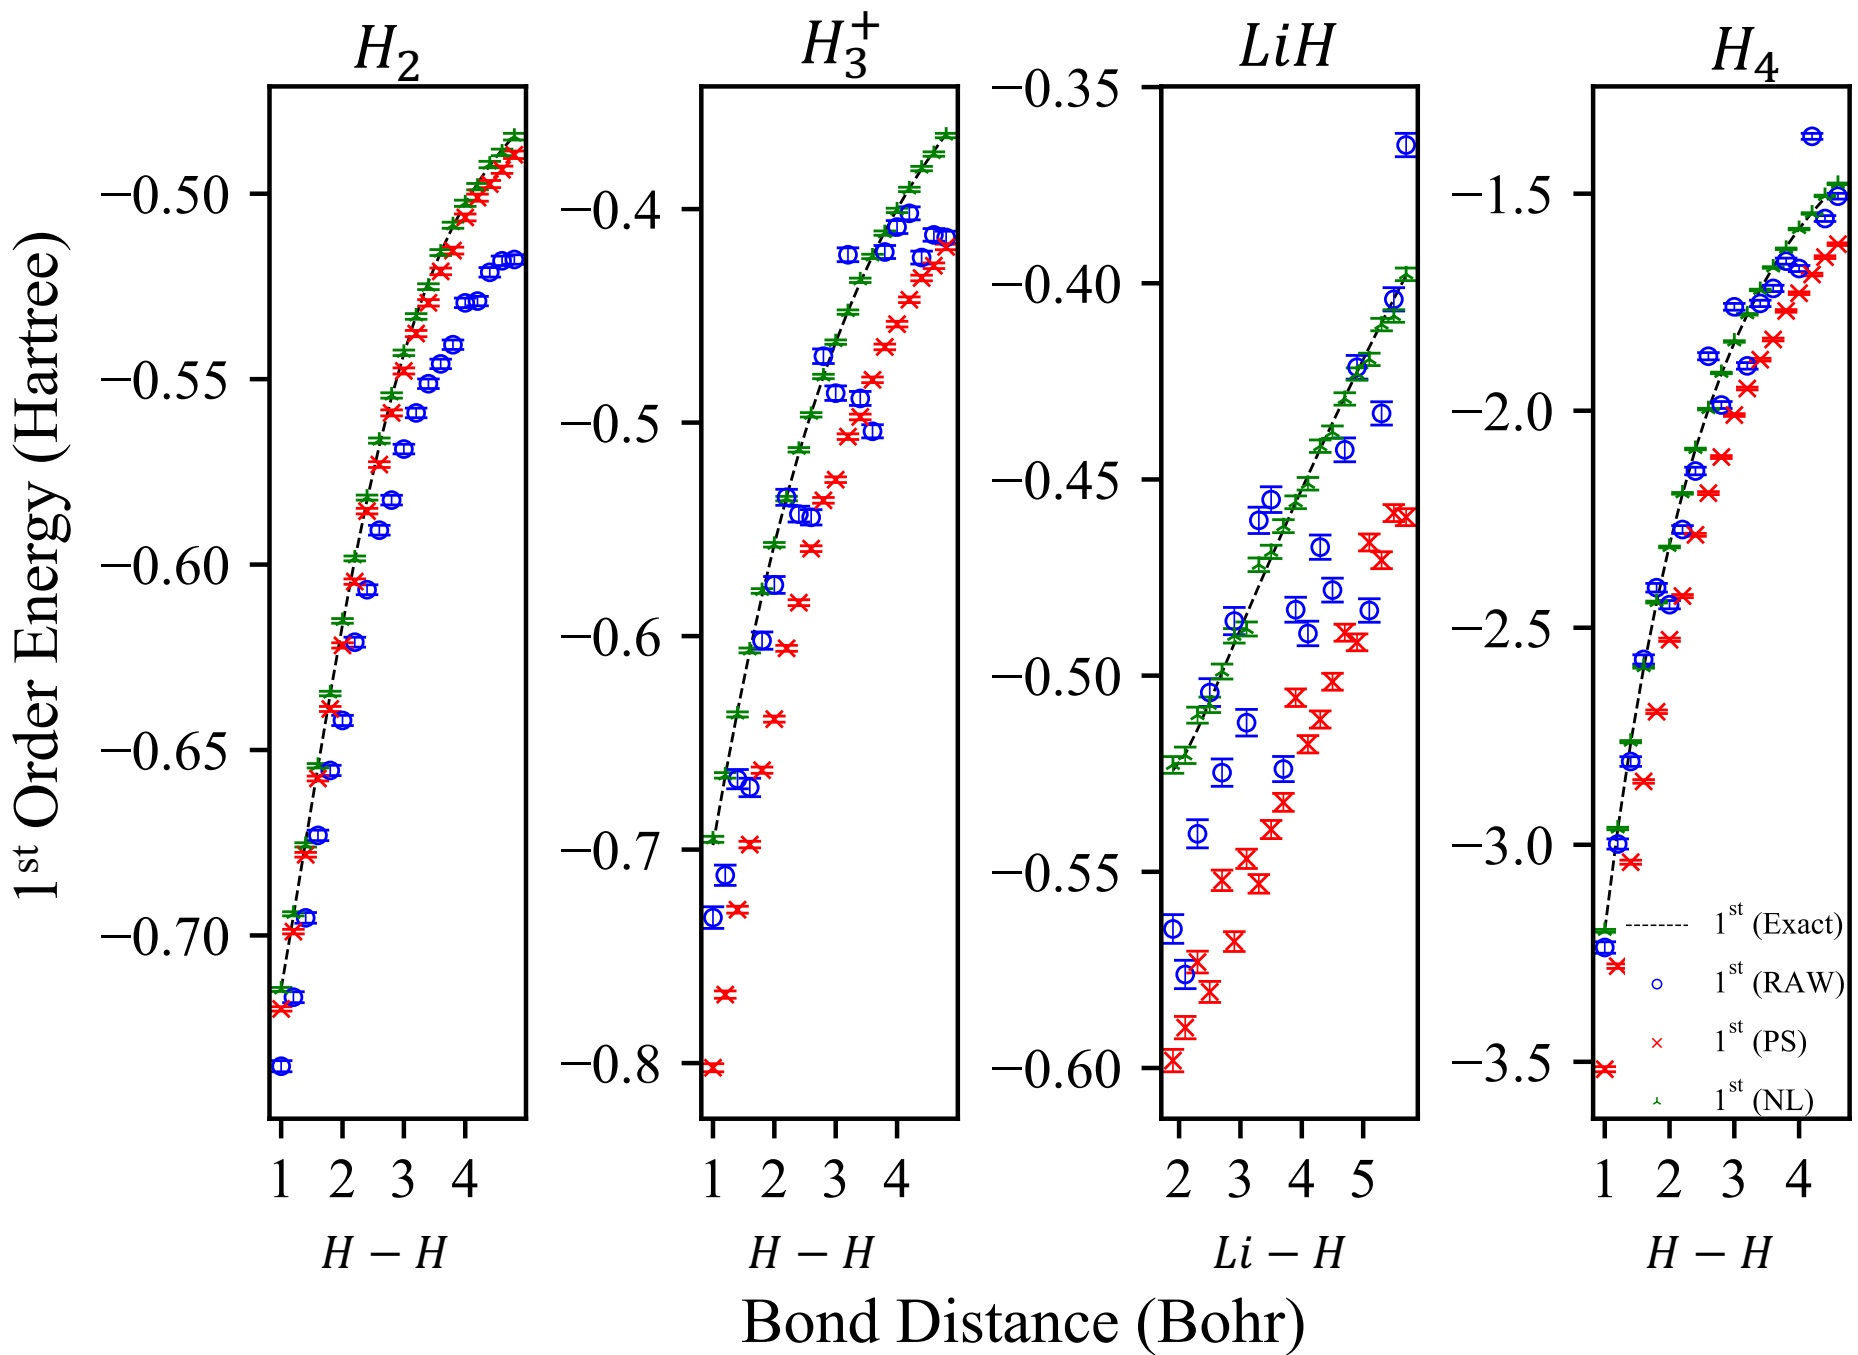

# Simulated IBM Auckland

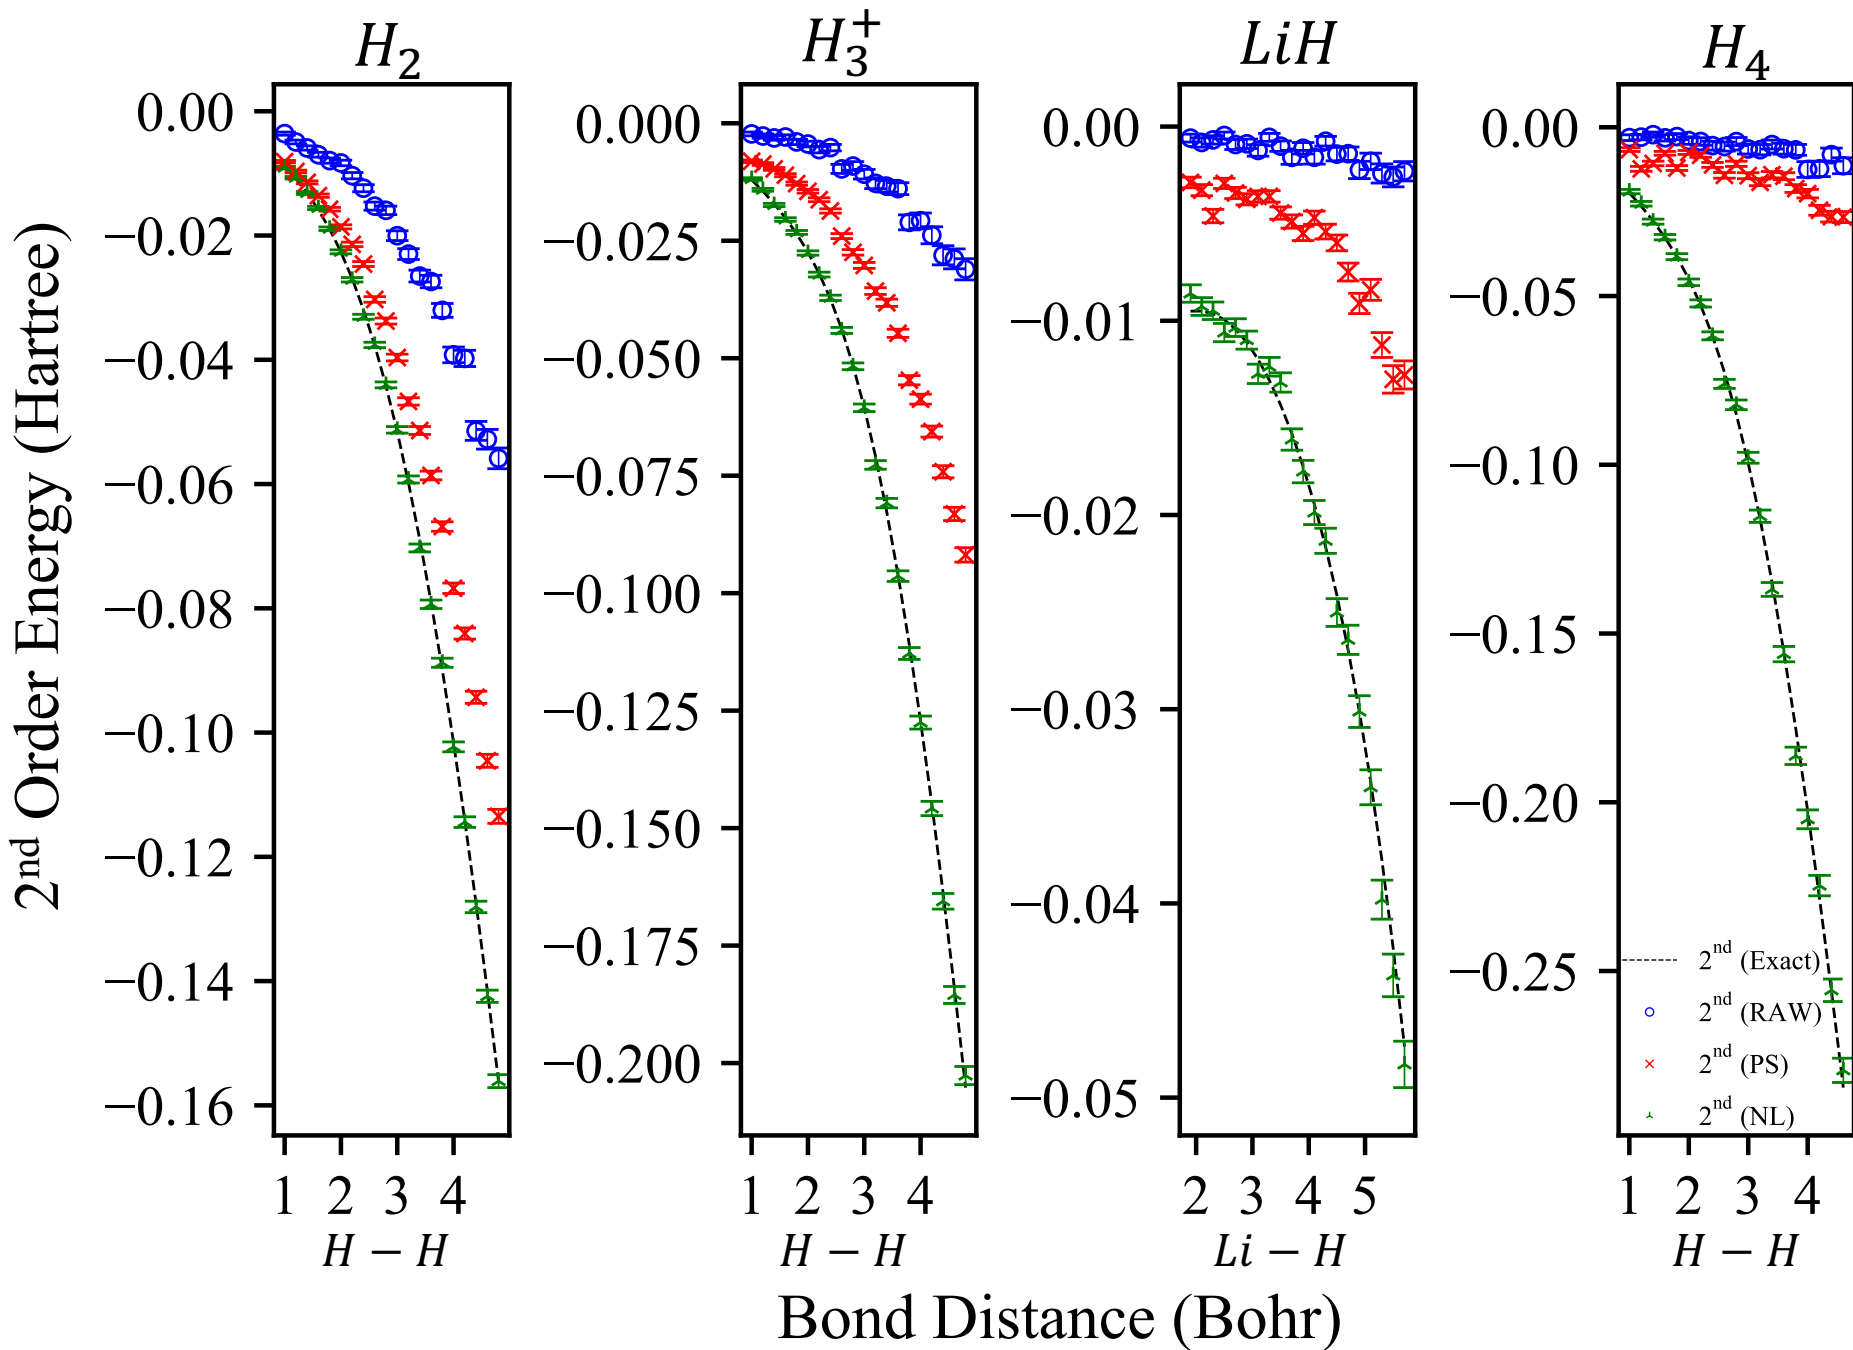

# $H_2$ Molecule

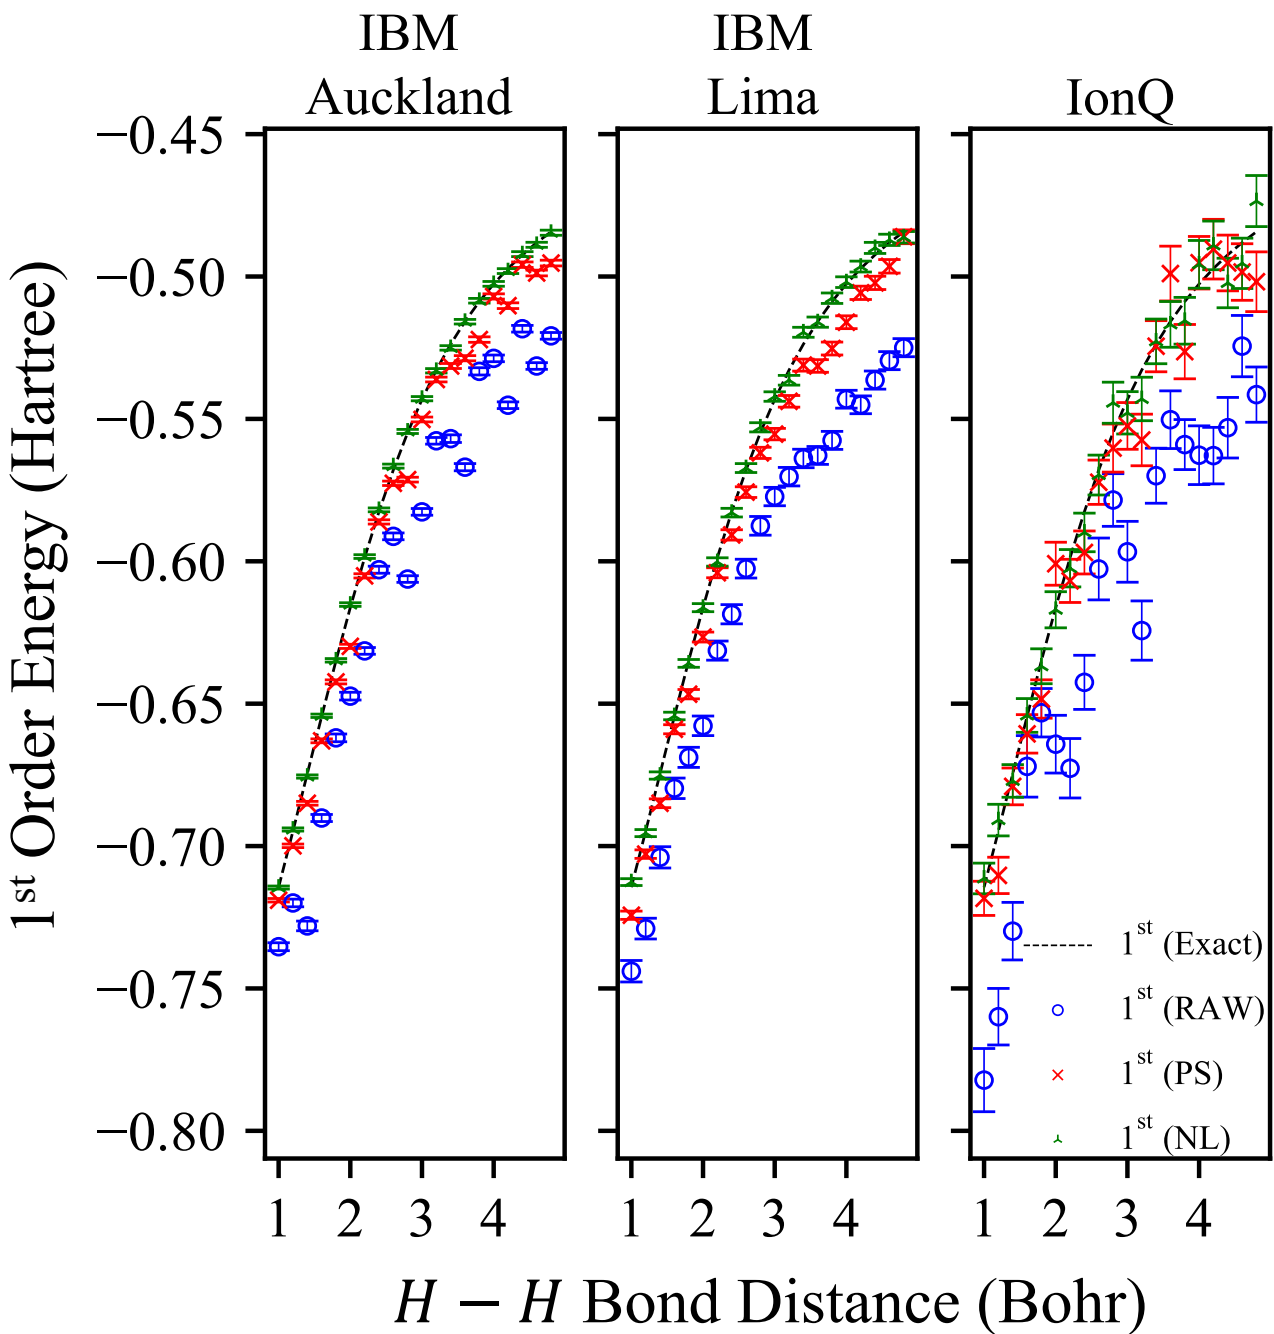

# $H_2$ Molecule

IBM  
Auckland

IBM  
Lima

IonQ

2<sup>nd</sup> Order Energy (Hartree)

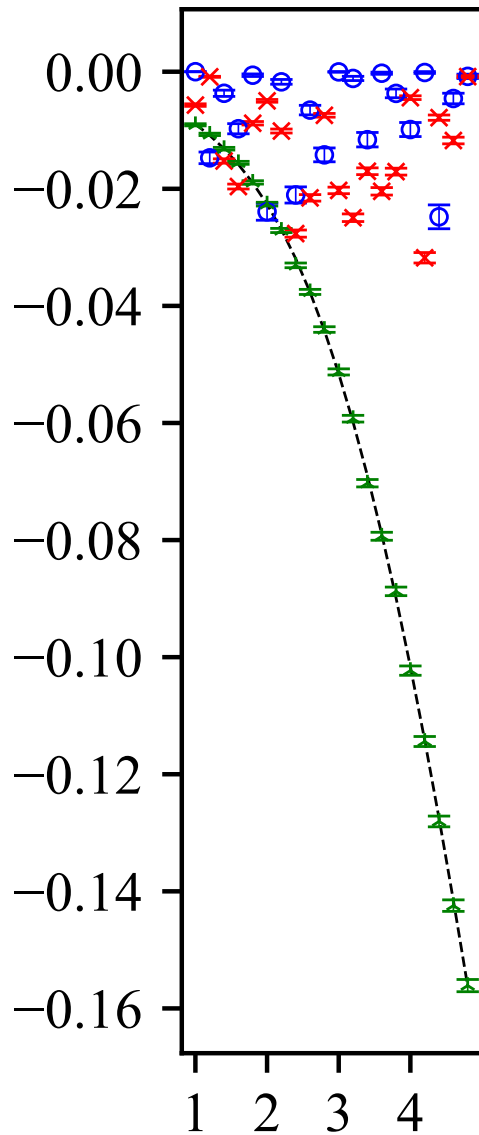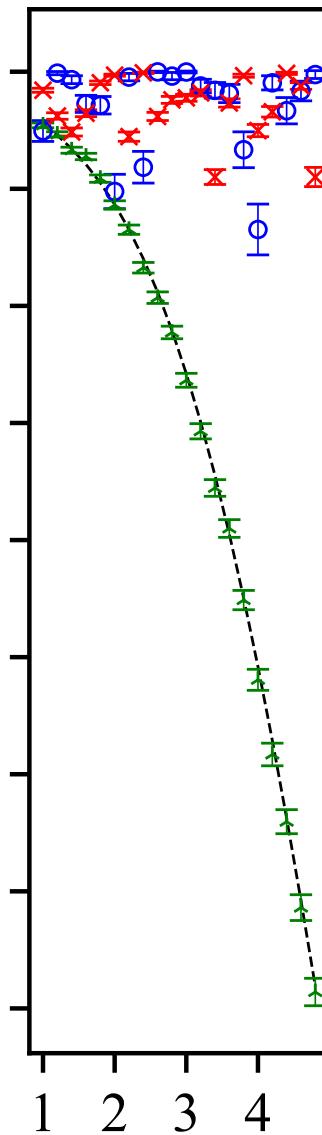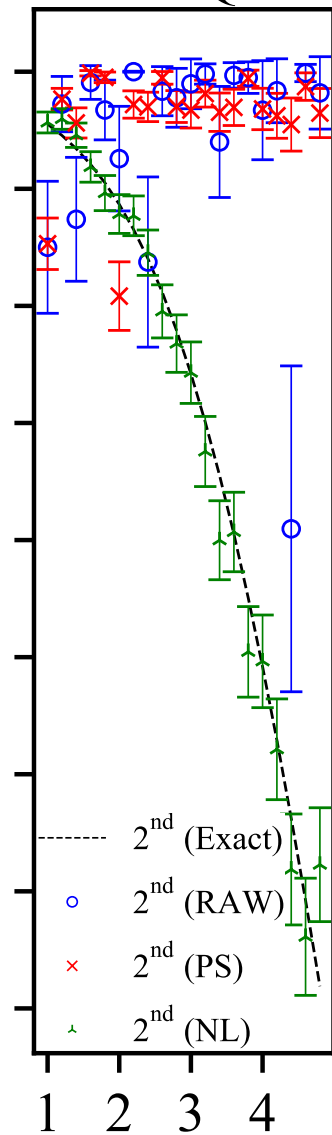

$H - H$  Bond Distance (Bohr)
